# Supplementary material for: Agent-based Learning of Materials Datasets from Scientific Literature
Source: arXiv:2312.11690 source file (2023-12-18)
Supplement: Supplementary file 1 [file ground-truth.tex]

% [inline block 0: 1 envs, 69789 chars -> data_tex | \begin{longtable}{lllll} \caption{Ground-truth water stability for a selection of 101 research articles.} \label{tab:gro...]
